# Supplementary material for: SneakySnake: A Fast and Accurate Universal Genome Pre-Alignment Filter for CPUs, GPUs, and FPGAs
Source: arXiv:1910.09020 source file (2020-11-23)
Supplement: Supplementary file 1 [file SneakySnakeSuppMaterials23Nov2020.pdf]

**Supplementary Materials**

## 5. Run Time and Space Complexity Analysis of the SneakySnake Algorithm

We analyze the asymptotic run time and space complexity of the SneakySnake algorithm. We provide the pseudocode of SneakySnake in Algorithm 1. The SneakySnake algorithm builds the chip maze on-the-fly by partially constructing each horizontal routing track starting from each new checkpoint until it reaches an obstacle in each horizontal routing track. The SneakySnake algorithm does not necessarily construct the entire chip maze. At each new checkpoint, the SneakySnake algorithm examines if the signal net 1) does not reach the destination terminal or 2) does not exceed the allowed propagation delay before the SneakySnake algorithm continues calculating the horizontal routing tracks (as we explain in Algorithm 1, line 4). It then uses the function *UpperHRT*() (Algorithm 2) to construct the first escape segment, after the current checkpoint, of each of the upper HRTs (as we explain in Algorithm 1, line 6). After constructing the escape segments, it computes their length and returns the length of the longest escape segment. Note that during the first iteration of the SneakySnake algorithm, the function *UpperHRT*() (Algorithm 2) returns a value of 1, which is the length of a single obstacle. This is because all upper HRTs start with an obstacle. The SneakySnake algorithm performs the same steps as in the function *UpperHRT*() for the main HRT (Algorithm 1, line 7) and the lower HRTs (Algorithm 1, line 12), by calling the two functions: *MainHRT*() (Algorithm 3) and *LowerHRT*() (Algorithm 4). Finally, we update the position of the checkpoint and the current propagation delay of the found signal net through Algorithm 1, lines 15-18. Once the signal net exceeds the allowed propagation delay, the SneakySnake algorithm terminates (as we show in Algorithm 1, line 4 and lines 19-20). Otherwise, the SneakySnake algorithm allows computationally expensive edit distance or pairwise alignment algorithms to compute their output based on the user-defined parameters (as we show in Algorithm 1, lines 21-22).

On the one hand, the lower-bound on the time complexity of the SneakySnake algorithm is $O(m)$, which is achieved when the SneakySnake algorithm reaches the destination terminal of the maze without facing any obstacle along the signal net. For example, when a query sequence matches exactly a reference sequence, the SneakySnake algorithm traverses only through the $E+1^{th}$ HRT (i.e., main HRT) and then allows the edit distance or alignment algorithm to perform its computation.

On the other hand, the upper-bound on the run time complexity of the SneakySnake algorithm is reached when the algorithm has to construct the *entire* chip maze, which is the worst case. As we have $2E+1$ horizontal routing tracks, each of which is $m$ characters long, the upper-bound run time complexity is $O((2E+1)m)$. However, it is unrealistic to construct the entire chip maze, as in this case, all the horizontal routing tracks should be identical in terms of the number and the location of all obstacles. Consider a pair of query and reference sequences, where each character is generated completely randomly (having 1/4 probability of being either A, C, G, or T). The probability that a character of the query sequence does not match any neighboring character of the reference sequence during the construction of any of the $2E+1$ horizontal routing tracks is $(3/4)^{2E+1}$, which decreases exponentially as $E$ increases. Therefore, this upper-bound on the run time complexity is still loose.

**Algorithm 1**: SneakySnake

**Input:** query (*Q*), reference (*R*), and edit distance threshold (*E*)

**Output:** -1 for dissimilar sequences / *EditDistance*() or *Alignment*()

**Functions:** *UpperHRT*(), *MainHRT*(), *LowerHRT*() construct the first escape segment of each of the *E* upper, main, and *E* lower horizontal routing tracks, respectively, and returns the length of the longest escape segment

**Pseudocode:**

```
checkpoint = 0
PropagationDelay = 0
m = length(Q)
while checkpoint < m and PropagationDelay <= E do
    count = 0
    longest_es = UpperHRT(Q[checkpoint:m-1], R[checkpoint:m-1], E)
    count = MainHRT(Q[checkpoint:m-1], R[checkpoint:m-1])
    if count == m then
        return = EditDistance() or Alignment()
    if count > longest_es then
        longest_es = count
    count = LowerHRT(Q[checkpoint:m-1], R[checkpoint:m-1], E)
    if count > longest_es then
        longest_es = count
    checkpoint = checkpoint + longest_es
    if checkpoint < m then
        PropagationDelay++
        checkpoint++
if PropagationDelay > E then
    return -1
else
    return EditDistance() or Alignment()   //depends on user's requirement
```

**Algorithm 2**: UpperHRT

**Input:** query (*Q[checkpoint:m-1]*), reference (*R[checkpoint:m-1]*), and edit distance threshold (*E*)

**Output:** length of the longest escape segment of the upper horizontal routing tracks

**Pseudocode:**

```
longest_es = 0
for r = E to 1 do
    count = 0
    for n = checkpoint to length(Q)-1 do
        if n < r then
            goto EXIT
        else if Q[n-r] != R[n] then
            goto EXIT
        else if Q[n-r] == R[n] then
            count++
EXIT:
    if count > longest_es
        longest_es = count
return longest_es
```

**Algorithm 3**: MainHRT

**Input:** query (*Q[checkpoint:m-1]*) and reference (*R[checkpoint:m-1]*)
**Output:** length of the longest escape segment of the main horizontal routing track
**Pseudocode:**

```
longest_es = 0
for n = checkpoint to length(Q)-1 do
    if Q[n] != R[n] then
        return longest_es
    else if Q[n] == R[n] then
        longest_es = longest_es + 1
return longest_es
```

**Algorithm 4**: LowerHRT

**Input:** query (*Q[checkpoint:m-1]*), reference (*R[checkpoint:m-1]*), and edit distance threshold (*E*)
**Output:** length of the longest escape segment of the lower horizontal routing tracks
**Pseudocode:**

```
longest_es = 0
for r = 1 to E do
    count = 0
    for n = checkpoint to length(Q)-1 do
        if n > m-r-1 then
            goto EXIT
        else if Q[n+r] != R[n] then
            goto EXIT
        else if Q[n+r] == R[n] then
            count++
EXIT:
    if count > longest_es
        longest_es = count
return longest_es
```

## 6. Proofs of the Correctness and Optimality of the SneakySnake Algorithm

As the propagation delay of a signal net is mainly affected by the number of obstacles that are considered in the horizontal escape segments of the selected path, for simplicity, we do not consider the vertical segments in our proof.

### 6.1. Correctness proof

PROOF. We prove Theorem 1 by contradiction. Let $A = \{s_1, s_2, \ldots, s_n\}$ be the signal net that connects the source terminal to the destination terminal using $n$ escape segments that are part of the horizontal routing tracks within a routing region. The escape segments are sorted by their start position (i.e., $s_1$ starts before $s_2$ and ends at $s_2$). Assume that the SneakySnake algorithm is not able to find this signal net $A$ that reaches the

destination terminal. This means that the SneakySnake algorithm finds an escape segment, $s_k$, but it fails to find the next escape segment, $s_{k+1}$. Since there is a signal net that connects $s_1$ to $s_n$, there exists an escape segment that starts before $s_{k+1}$ and ends at $s_{k+1}$. This escape segment is not reachable from $s_k$ (as we assume that the SneakySnake algorithm terminates the solution after finding $s_k$), so it should be reachable from another escape segment, $s_t$, where $t < k$. This indicates that $s_{k+1}$ is not reachable from $s_k$ and $s_k$ is not reachable from $s_t$. This contradicts the assumption that $s_{k+1}$ is reachable and it is part of the solution. Thus, our assumption that the SneakySnake algorithm is not able to find a signal net is wrong. ■

### 6.2. Optimality proof

PROOF. We prove Theorem 2 by induction. Suppose you have a set of $n$ candidate horizontal segments {1, 2, …, $n$} that are part of the horizontal routing tracks within a routing region. Each horizontal segment has a pair of start and end positions ($s(i)$, $f(i)$). The SneakySnake algorithm determines a signal net with the minimum total propagation delay by repeatedly selecting from the available horizontal segments the one that starts at the current location and has the farthest end location, and removing all overlapping horizontal segments from the set. Let $A = \{x_1, x_2, \ldots, x_k\}$ be the solution (set of escape segments) to SNR problem provided by the SneakySnake algorithm. The escape segments are sorted by their start position (i.e., $x_1$ starts before $x_2$ and ends at $x_2$). Let $B = \{y_1, y_2, \ldots, y_m\}$ be the optimal solution for the same SNR problem. Let $k = |A|$ and $m = |B|$ denote the number of escape segments in $A$ and $B$, respectively. The proof is by *induction* on the number of escape segments. We will compare $A$ and $B$ by their segments' end positions. We will show that for all $r \leq k$, $f(x_r) \geq f(y_r)$.

As the base case, we take $k = m = 1$. Since SneakySnake and the optimal algorithm select the longest escape segment that start at the beginning of a horizontal routing track, it certainly must be the case that $f(x_1) \geq f(y_1)$.

For $r > 1$, assume the statement $f(x_{r-1}) \geq f(y_{r-1})$ is true for $r - 1$ and we will prove it for $r$. The induction hypothesis states that $f(x_{r-1}) \geq f(y_{r-1})$, and so any horizontal segment that is not overlapping with the first $r - 1$ escape segments in the optimal solution is certainly not overlapping with the first $r - 1$ escape segments of the SneakySnake algorithm. Therefore, we can add $y_r$ to the SneakySnake solution, and since the SneakySnake algorithm always considers the longest escape segments, it must be the case that $f(x_r) \geq f(y_r)$. So we have that for all $r \leq k$, $f(x_r) \geq f(y_r)$. In particular, $f(x_k) \geq f(y_k)$. If $A$ is not optimal, then it must be the case that $m < k$, and so there is an escape segment $x_{m+1}$ in $A$ that is not in $B$. This escape segment must start after $A$'s $m^{th}$ escape segment ends, and hence after $f(y_m)$. But then the segment $x_{m+1}$ is not overlapping with all the escape segments in $B$, and so it should be part of the solution in $B$. This contradicts the assumption that $m<k$, and thus $A$ has as many elements as $B$. So the SneakySnake algorithm always produces an optimal solution. ■

## 7. Similarities and Differences Between the SNR Problem in VLSI CAD and the SNR Problem for Pre-alignment Filtering

We use the SNR problem as a simple example that can explain/visualize the pre-alignment filtering problem (Alser *et al.*, 2020a; Alser *et al.*, 2020b). We believe that the SNR problem and the pre-alignment filtering problem are very similar. There are three main similarities. 1) Both problems aim to find the net (a set of non-overlapping matching segments) that provides the minimal propagation delay (number of edits). 2) Both problems have normally a free choice of pin assignment. That is, the source and destination nodes can be any of the IO pads around the chip. 3) Both problems consider the presence of obstacles (edits) and some constraints. Fig. 6 provides a 3-dimensional top-view and a side-view of the chip maze in Fig. 1 to clearly illustrate how the different metal layers (routing tracks) are connected.

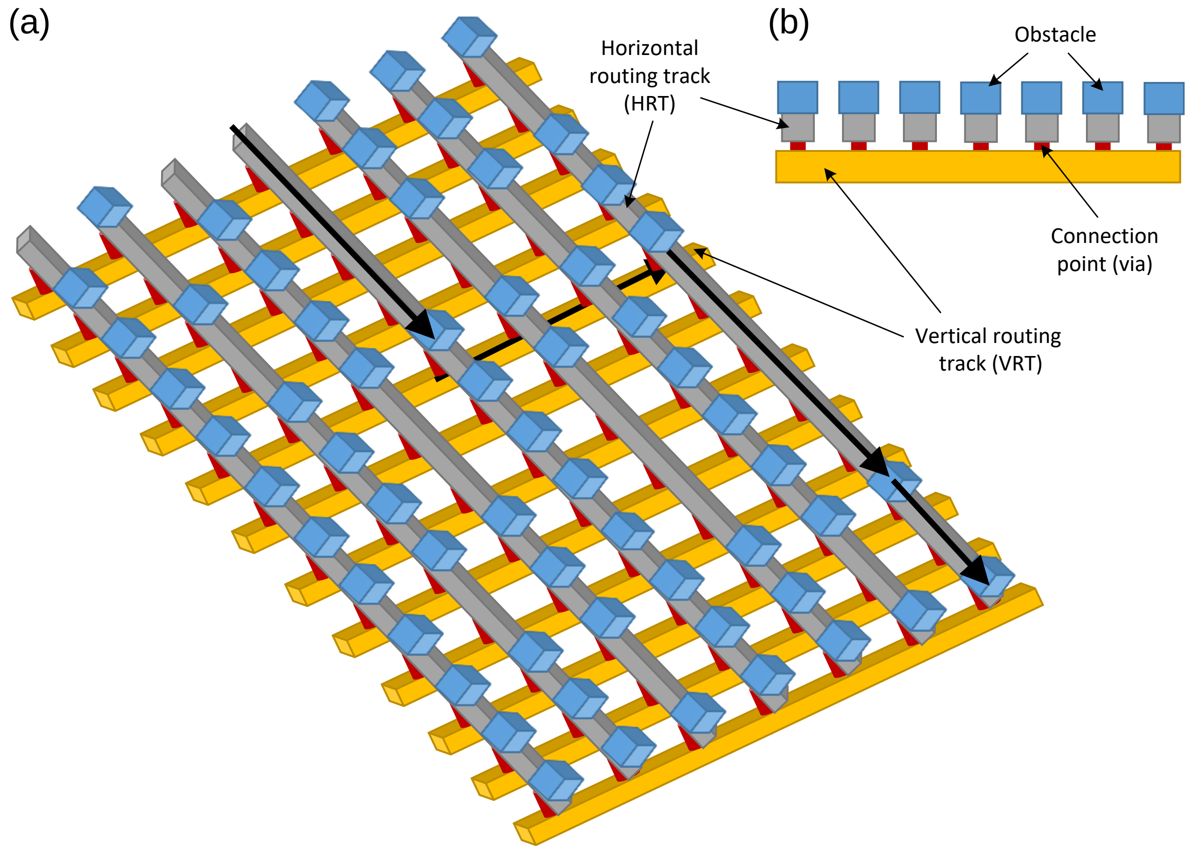


**Fig. 6: (a) A 3-dimensional top-view and (b) side-view of the same chip maze presented in Fig. 1. The signal net has 3 obstacles, each of which is located at the end of each escape segment (a black arrow on the horizontal routing track).**

However, we also highlight four key differences that make our SNR problem slightly different (a special case) from what we normally have in VLSI CAD, as we summarize in Table 2. These four differences can render the existing general algorithms that solve the SNR problem in VLSI CAD, e.g., (Roy and Markov, 2008; Chu and Wong, 2007) inefficient at directly solving our SNR problem. Instead, SneakySnake provides a new efficient algorithm that does not require building the entire chip maze in advance (as we illustrate in Fig. 2(c)), while it considers the propagation delay of each obstacle faced throughout the signal net.

**Table 2: A summary of the four key differences between the SNR problem in VLSI CAD and the SNR problem for pre-alignment filtering.**

| | **SNR problem in VLSI CAD** | **SNR problem for pre-alignment filtering** |
|---|---|---|
| **The size and location of an obstacle** | The obstacles (modules such as caches, embedded memories, and intellectual property (IP) cores) in the VLSI chip do not necessarily have the same shape, area, nor fixed locations. | In our chip maze, all obstacles are assumed to be 1x1 objects and can be placed anywhere in the grid. |
| **Optimal solution** | The obstacle that is faced by the optimal net is typically avoided in VLSI routing, using a new metal layer or another track, if available, on the same metal layer. | The obstacle that is faced throughout the optimal net cannot be avoided and it contributes to the total delay of the optimal net. |
| **Pre-processing requirements** | Prior to solving the SNR problem, a step called *chip planning* should be carried out to optimize the location and the aspect ratio of each individual obstacle. | No pre-processing steps are required. |
| **Building a complete chip maze** | After performing chip planning, we build a complete graph that represents the chip maze and then apply one of the state-of-the-art algorithms (e.g., Dijkstra's algorithm (Dijkstra, 1959) and A* (Hart *et al.*, 1968) to solve the SNR problem. These algorithms typically require building the entire chip maze and calculating the distance between every two nodes before applying the algorithm itself. A detailed summary of these algorithms is presented in (Roy and Markov, 2008; Chu and Wong, 2007). | SneakySnake builds only the portion of the chip maze that is absolutely needed to provide an optimal solution to the SNR problem for pre-alignment filtering. |

## 8. Snake-on-Chip Hardware Architecture

Next, we present the details of our hardware architecture of Snake-on-Chip in four key steps.

(1) Snake-on-Chip constructs the *entire* chip maze of each subproblem. Each chip maze has 2$E$+1 bit-vectors (rows) and each bit-vector is $t$ bits long. This is different from the CPU implementation of the SneakySnake algorithm, as the number of entries computed in each row is no longer limited to the entries that are located only between a checkpoint and the first following obstacle. This is due to the fundamental difference between a CPU core (sequential execution) and an FPGA chip (parallel processing). We want to concurrently compute all bits of all bit-vectors beforehand so that we can exploit massive bitwise parallelism provided by an FPGA and perform computations on all bit-vectors in a parallel fashion.

(2) It computes the length of the first horizontal segment of consecutive zeros for each bit-vector (i.e., each HRT) using a leading-zero counter (LZC). Snake-on-Chip uses the LZC design proposed in (Dimitrakopoulos *et al.*, 2008) as it requires a low number of both logic gates and logic levels. It counts the number of leading consecutive zeros that appear in a $t$-bit input vector.

(3) Snake-on-Chip finds the bit-vector (i.e., HRT) that has the largest number of leading zeros. Snake-on-Chip implements a hierarchical comparator structure with $\lceil log_2(2E+1) \rceil$ levels. Each comparator compares the output of two LZCs and finds the largest value. That is, we need 2$E$+2 comparators, each of which is a ($\lfloor log_2 t \rfloor + 1$)-bit comparator, for comparing the leading zero counts of 2$E$+1 $t$-bit LZCs and finding the largest leading zero count. Consider that we choose $t$, $E$, and $m$ to be 8 columns, 5 edits (i.e., 11 rows), and 100 characters, respectively. This results in partitioning the chip maze of size 11 × 100 into 13 (i.e., $m$/$t$) subproblems, each of size 11 × 8. We need 11 LZCs and 12 comparators. We arrange the 12 LZC comparators into 4 levels: the first level of LZC comparators that is directly connected to the LZCs has 6 LZC comparators, the second level has 3 LZC comparators, the third level has 2 LZC comparators, and the last level has a single LZC comparator. This hierarchical comparator structure compares the 11 escape segments of a subproblem and produces the length of the longest escape segment ($x$). We provide the overall architecture of the 4-level LZC comparator tree including the 11 LZC block diagrams in Fig. 7.

(4) After computing the length of the longest segment (i.e., the largest leading-zero count), Snake-on-Chip creates a new checkpoint to iterate over the HRTs once again to find the next optimal escape segment. Snake-on-Chip achieves this by shifting the bits of each row (i.e., HRT) to the right-hand direction (assuming the least significant bit starts from the right-hand side). The shift amount is equal to $x$ bits, where $x$ is the length of the found longest escape segment of the consecutive zeros calculated in the third step. To skip the obstacle that exists at the end of the longest escape segment, Snake-on-Chip shifts the bits of each row by an additional single step to the right-hand direction. This guarantees to exclude the previously-found longest escape segment along with a single obstacle from the new search round.

(5) Snake-on-Chip repeats the previous three steps (steps 2, 3, and 4) to find the next optimal escape segment starting from the least significant bit (i.e., the new checkpoint) all the way to the most significant bit. Repeating the previous three steps for each iteration is achieved by building a new module instance for the architecture design of all the three previous steps. The 2$E$+1 output bit-vectors calculated by the fourth step are the 2$E$+1 input bit-vectors to the new hardware instance. The number of iterations ($y$, i.e., hardware instances) needed depends on the desired accuracy of the SneakySnake algorithm (as we experimentally

evaluate the effect of choosing different values of $y$ on the accuracy of Snake-on-Chip in https://github.com/CMU-SAFARI/SneakySnake/tree/master/Evaluation%20Results). If our target is to find an optimal signal net that has at most a single obstacle within each subproblem built in the first step, then we need to build two hardware instances, each of which performs the previous three steps (steps 2, 3, and 4). For example, let $D$, one of the $2E+1$ bit-vectors that is also the optimal signal net, be "00010000", where $t = 8$. The first hardware instance computes the value of $x$ (the length of the longest escape segment calculated in the third step) as four zeros, updates the bits of $D$ to "11111000", and passes the updated $D$ to the second hardware instance. The second hardware instance computes the value of $x$ as three zeros and updates the bits of $D$ to "11111111".

(6) The last step is to calculate the total number of obstacles faced along the entire optimal signal net in each subproblem. For each subproblem, Snake-on-Chip calculates the total number of obstacles as follows:

$$min\ (y, t - \sum_{k=1}^{y} x_k) \qquad (2)$$

where $y$ is the total number of hardware instances included in the architecture of Snake-on-Chip, $t$ is the width of the chip maze of each subproblem, and $x_k$ is the length of the longest segment of consecutive zeros found by the hardware instance of index $k$. Hence, the total number of obstacles for the original problem of size $(2E+1) \times m$ is simply the summation of the total number of obstacles (calculated in Equation 2) faced along the optimal signal net of all subproblems.

Snake-on-Chip makes the following technical contributions:

1) We introduce the approach of dividing a single SNR problem into several subproblems that can be solved concurrently and independently. FPGAs typically provide parallelism in two main ways: 1) providing a large number (typically few millions) of look-up tables (LUTs) that can form a large number of hardware compute units to perform computation in a parallel fashion and 2) providing massive bitwise parallelism for each compute unit. To build Snake-on-Chip, we need to decide on 1) the size and the number of compute units (we call them *filtering units*) that can be integrated within the FPGA chip and 2) custom-tailored operations to the SNR problem that leverage bitwise operations. A filtering unit that occupies a large number of LUTs can have a large critical path delay, which directly affects the maximum operating frequency and hence it affects the filtering speed. The approach of dividing the SNR problem into several SNR subproblems provides three key benefits that can reduce the LUT requirement of each filtering unit, as we list in Section 2.5 in the main manuscript.
2) We comprehensively analyze and evaluate different design choices for the size of each filtering unit of Snake-on-Chip (as we experimentally evaluate in "Effect of $y$ & $t$ on SneakySnake" Excel sheet in https://github.com/CMU-SAFARI/SneakySnake/tree/master/Evaluation%20Results). This analysis helps us to build an efficient hardware architecture that has a very small LUT requirement. This allows integrating a large number of these hardware filtering units within the FPGA chip, where they all operate concurrently and independently.
3) We build a modular hardware architecture that is scalable with both sequence length and edit distance threshold.

4) We introduce an efficient FPGA-friendly implementation with a low FPGA resource utilization (less than 1.5% of the total number of FPGA LUTs for a single filtering unit, as we show in Section 10.4 in the Supplementary Materials). We make both the hardware architecture of Snake-on-Chip and the complete software/hardware co-design FPGA project publicly available at: https://github.com/CMU-SAFARI/SneakySnake/tree/master/Snake-on-Chip

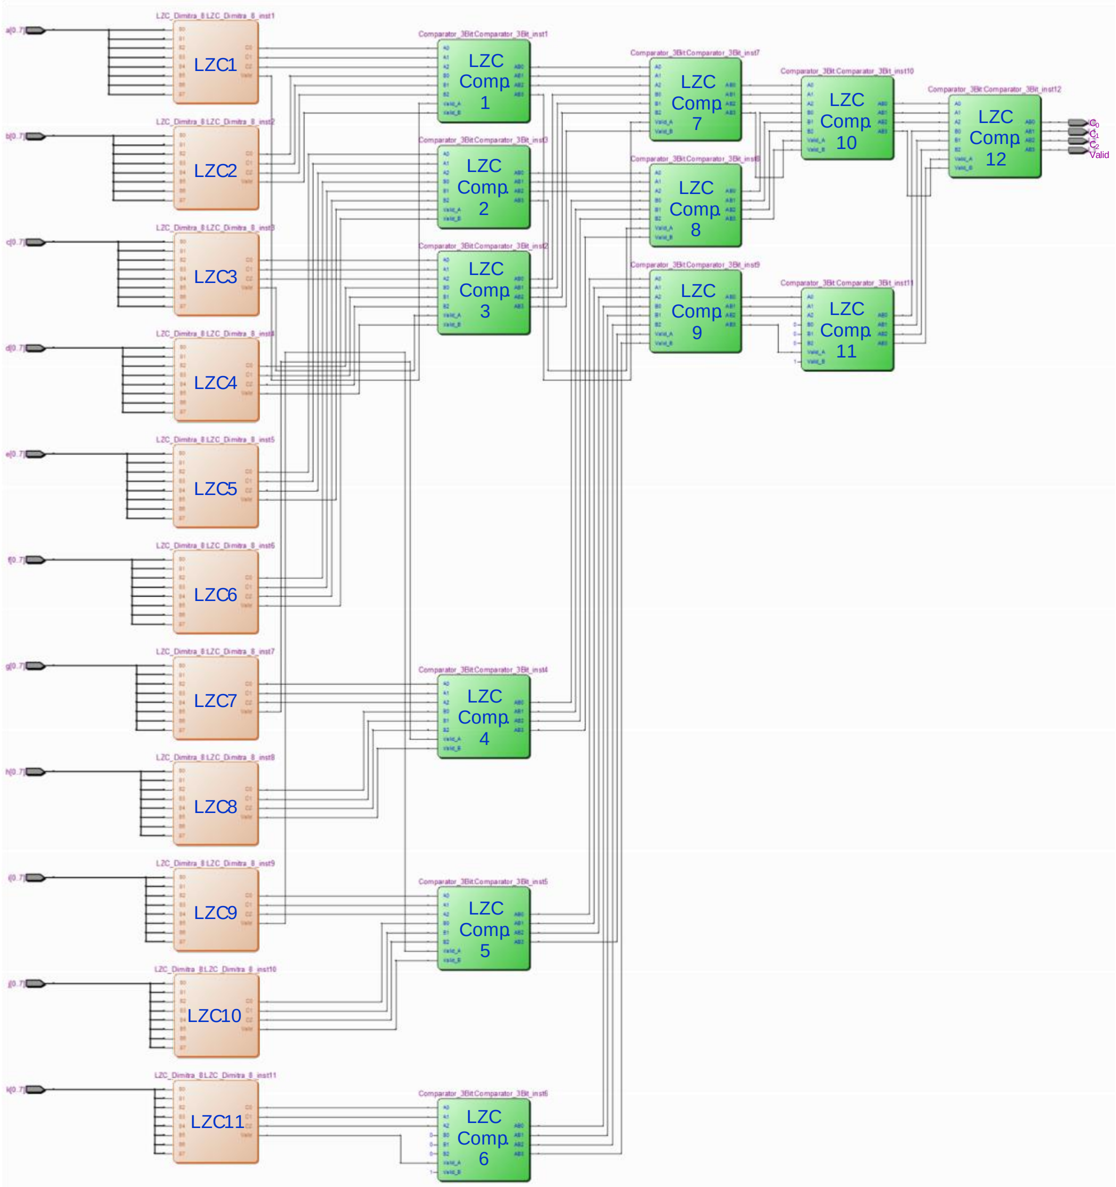


**Fig. 7: Block diagram of the 11 LZCs (highlighted in orange color) and the hierarchical LZC comparator tree (highlighted in green color) for computing the largest number of leading zeros in 11 rows.**

## 9. Snake-on-GPU Parallel Implementation

Snake-on-GPU makes three key assumptions that help with providing an efficient GPU implementation. (1) The entire input dataset of query and reference sequences fits in the GPU global memory, which is the off-chip DRAM memory of a GPU (NVIDIA, 2019a) and it typically fits several GB of data (e.g., NVIDIA GeForce RTX 2080Ti card, which is used for Snake-on-GPU implementation, has a global memory of 11 GB). (2) We copy the entire input dataset from the CPU main memory to the GPU global memory before the GPU kernel execution starts. This enables massively-parallel computation by making a large number of input sequences available in the GPU global memory. (3) We copy back the pre-alignment filtering results from the GPU global memory to the CPU main memory only after the GPU kernel completes the computation. If the size of the input dataset exceeds the size of the GPU global memory, we divide the dataset into independent smaller datasets, each of which can fit the capacity of the GPU global memory. This approach also helps us to overlap the computation performed on one small dataset with the transfer of another small dataset between the CPU memory and GPU memory (Gómez-Luna *et al.*, 2012).

Given the large size of the input dataset that the GPU threads need to access from the GPU global memory, we carefully design Snake-on-GPU to efficiently use the on-chip register file to store the query and the reference sequences and avoid unnecessary accesses to the off-chip global memory. The workflow of Snake-on-GPU includes two key steps, as we show in Fig. 8. 1) Each thread copies a single reference sequence and another single query sequence from global memory to the on-chip registers. Assuming the maximum length of a query (or reference) sequence is $m$ (i.e., the maximum number of VRTs), we need $2m$ bits to encode each character of the query (or reference) sequence into a unique binary representation. Since the size of a register is 4 bytes (32 bits), each thread needs $R = \left\lceil \frac{2m}{32} \right\rceil$ registers to store an entire query/reference sequence. For example, for a maximum length of $m$ = 128, $R$ = 8. This way, 16 registers are enough to store both query and reference sequences. This number is much lower than the maximum of 256 registers that each thread can use in current NVIDIA GPUs. Thus, the resources of a GPU core are not exhausted and more threads can run concurrently. 2) Each thread solves the complete SNR problem for a single query sequence and a single reference sequence. Each GPU thread applies the same computation of the SneakySnake algorithm to solve the SNR problem.

Snake-on-GPU makes the following two technical contributions:

1) We provide a theoretical analysis of the available resources (on-chip register file and off-chip global memory) of typical modern GPUs and how they affect the performance of Snake-on-GPU in Section 9. Based on this analysis, Snake-on-GPU uses one single GPU thread to solve one SNR problem. This design choice provides three key benefits: 1) it maximizes the utilization of the on-chip registers as they provide fast data access, 2) it minimizes the utilization of the off-chip global memory as off-chip communication is expensive, i.e., time-consuming and energy inefficient (Mutlu *et al.*, 2019; Ghose *et al.*, 2019), and it can affect the number of threads that operate concurrently (NVIDIA, 2019a), and 3) it avoids the need for synchronizing several threads working on the same SNR problem. These benefits lead to achieving a high degree of parallelism.
2) We introduce an efficient fully-configurable GPU implementation where users can change the edit distance threshold value at run time without the need to change the implementation. We make our parallel GPU implementation, Snake-on-GPU, *publicly available* at: https://github.com/CMU-SAFARI/SneakySnake/blob/master/Snake-on-GPU

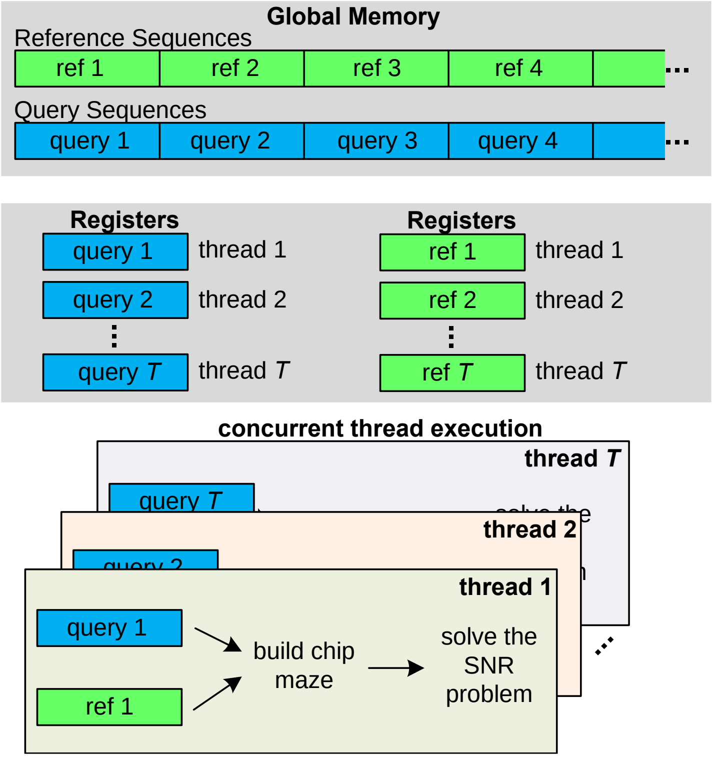


**Fig. 8: Workflow of Snake-on-GPU. It includes two key steps: (1) each GPU thread loads a single reference sequence and a single query sequence into registers, (2) the assigned thread solves a single SNR problem for the two sequences.**

## 10. Supplementary Evaluation

### 10.1. Dataset Descriptions

We have two key approaches to generating sequence pairs for testing the performance of pre-alignment filters. 1) We can use existing read mappers to find reference segments that might be similar or dissimilar to real reads. We use the reference segments that are generated by read mapper before applying the DP-based pairwise alignment step to ensure that we obtain both similar and dissimilar (i.e., that are usually filtered out by the pairwise alignment step) generated pairs (a read sequence and its reference segment). 2) We can also use available read simulators to generate sequence pairs. The read simulators allow controlling the type of edits, the number of edits, and their distribution over a sequence. We follow both approaches, as they both are still widely-used in evaluating existing algorithms (Li, 2018). Our experimental evaluation uses 4 different real datasets and 2 simulated datasets.

**Real datasets.** Each real dataset contains 30 million real sequence pairs (text and query pairs). We obtain two different read sets, ERR240727_1 and SRR826471_1, of the whole human genome that include two different read lengths, 100 bp and 250 bp, respectively. We download these two read sets from EMBL-

ENA (https://www.ebi.ac.uk/ena). We map each read set to the human reference genome (GRCh37) using the mrFAST mapper (Alkan *et al.*, 2009) and observe all potential mapping locations of every read. We obtain the human reference genome from the 1000 Genomes Project (1000 Genomes Project Consortium, 2015). Before mapping the reads, we disable the DP-based pairwise alignment algorithm of the mrFAST mapper to obtain both aligned and unaligned sequences. For each read set, we use two different maximum numbers of allowed edits (2 and 40 for *m* =100 bp and 8 and 100 for *m* = 250 bp) using the *e* parameter of mrFAST to generate four real datasets in total. Each dataset contains the sequence pairs that are generated by the mrFAST mapper before the read alignment step of mrFAST, such that we allow each dataset to contain both similar (i.e., having edits fewer than or equal to the edit distance threshold) and dissimilar (i.e., having more edits than the edit distance threshold) sequences over a wide range of edit distance thresholds. For the reader's convenience, we refer to these datasets as 100bp_1, 100bp_2, 250bp_1, and 250bp_2. We summarize the details of these four datasets in Table 3. We provide the source used to obtain the read sets, the read length in each read set, and the configuration used for the *e* parameter of mrFAST (Alkan *et al.*, 2009) for our real 4 datasets. We use Edlib (Šošić and Šikić, 2017) to assess the number of similar (i.e., having edits fewer than or equal to the edit distance threshold) and dissimilar (i.e., having more edits than the edit distance threshold) pairs for each of the 4 datasets across different user-defined edit distance thresholds. We provide these details for 100bp_1, 100bp_2, 250bp_1, and 250bp_2 in Table 4.

**Simulated datasets.** We generate two sets (we refer to them as 10Kbp and 100Kbp) of long sequence pairs using PBSIM (Ono *et al*., 2013). We choose this simulator as it provides pairs of two sequences, the original segment of the reference (not only the location as in some read simulators) and its simulated segment. This helps us to directly obtain sequence pairs that can be used to evaluate the performance of sequence aligners and pre-alignment filters. We use the first Human chromosome sequence (GRCh38.p13 assembly, downloaded from https://www.ncbi.nlm.nih.gov/nuccore/NC_000001.11) for the input reference sequence in PBSIM. We generate 10Kbp to have 100,000 sequence pairs, each of which is 10 Kbp long, at 30× genome coverage. 100Kbp has 74,687 sequence pairs, each of which is 100 Kbp long, at 30× genome coverage. For both sets (10Kbp and 100Kbp), we use the default error profile for continuous long reads (CLR) in PBSIM.

**Table 3: Benchmark Illumina datasets (read-reference pairs). We map each read set to the human reference genome to generate four datasets of sequence pairs (read sequence and reference segment) using different edit distance thresholds (using the *e* parameter).**

| **Accession no.** | **ERR240727_1** | | **SRR826471_1** | |
|---|---|---|---|---|
| **Source** | https://www.ebi.ac.uk/ena/data/view/ERR240727 | | https://www.ebi.ac.uk/ena/data/view/SRR826471 | |
| **Sequence Length** | 100 | | 250 | |
| **Sequencing Platform** | Illumina HiSeq 2000 | | Illumina HiSeq 2000 | |
| **Dataset** | 100bp_1 | 100bp_2 | 250bp_1 | 250bp_2 |
| **mrFAST *e*** | 2 | 40 | 8 | 100 |
| **Amount of Edits** | Low-edit | High-edit | Low-edit | High-edit |

**Table 4: Details of evaluating the number of similar and dissimilar sequences in each of our four datasets using Edlib over a wide range of edit distance thresholds of *E*= 0% up to *E*= 10% of the sequence length. Each dataset contains 30 million sequence pairs.**

| | 100bp_1 | | 100bp_2 | | | 250bp_1 | | 250bp_2 | |
|---|---|---|---|---|---|---|---|---|---|
| ***E* (%)** | **Similar** | **Dissimilar** | **Similar** | **Dissimilar** | ***E* (%)** | **Similar** | **Dissimilar** | **Similar** | **Dissimilar** |
| **0** | 381,901 | 29,618,099 | 11 | 29,999,989 | **0** | 707,517 | 29,292,483 | 49 | 29,999,951 |
| **1** | 1,345,842 | 28,654,158 | 18 | 29,999,982 | **1** | 1,462,242 | 28,537,758 | 163 | 29,999,837 |
| **2** | 3,266,455 | 26,733,545 | 24 | 29,999,976 | **2** | 1,973,835 | 28,026,165 | 301 | 29,999,699 |
| **3** | 5,595,596 | 24,404,404 | 27 | 29,999,973 | **3** | 2,361,418 | 27,638,582 | 375 | 29,999,625 |
| **4** | 7,825,272 | 22,174,728 | 29 | 29,999,971 | **4** | 3,183,271 | 26,816,729 | 472 | 29,999,528 |
| **5** | 9,821,308 | 20,178,692 | 34 | 29,999,966 | **5** | 3,862,776 | 26,137,224 | 520 | 29,999,480 |
| **6** | 11,650,490 | 18,349,510 | 83 | 29,999,917 | **6** | 4,915,346 | 25,084,654 | 575 | 29,999,425 |
| **7** | 13,407,801 | 16,592,199 | 177 | 29,999,823 | **7** | 5,550,869 | 24,449,131 | 623 | 29,999,377 |
| **8** | 15,152,501 | 14,847,499 | 333 | 29,999,667 | **8** | 6,404,832 | 23,595,168 | 718 | 29,999,282 |
| **9** | 16,894,680 | 13,105,320 | 711 | 29,999,289 | **9** | 6,959,616 | 23,040,384 | 842 | 29,999,158 |
| **10** | 18,610,897 | 11,389,103 | 1,627 | 29,998,373 | **10** | 7,857,750 | 22,142,250 | 1,133 | 29,998,867 |

## 10.2. Effect of Multithreading on Filtering and Alignment Time

We examine the execution time of SneakySnake, Parasail (Daily, 2016), and SneakySnake integrated with Parasail as the number of threads increases from 1 to 40, as we show in Fig. 9. We run this experiment using a 2.3 GHz Intel Xeon Gold 5118 CPU with up to 48 threads and 192 GB RAM. We choose SneakySnake as it is the only pre-alignment filter that supports multithreading, compared to Shouji (Alser *et al.*, 2019), MAGNET (Alser *et al.*, 2017b), GateKeeper (Alser *et al.*, 2017a), and SHD (Xin *et al.*, 2015). We choose Parasail (*parasail_nw_banded*) as it supports both multithreading and configurable scoring function. We make three key observations based on Fig. 9. (1) SneakySnake is always faster than Parasail over a wide range of both number of threads and datasets. SneakySnake is 9.3× (using 100bp_2 and 24 threads) to 30× (using 100bp_1 and a single thread) faster than Parasail in examining the sequence pairs, when the edit distance threshold is set to 10% of the sequence length. (2) The addition of SneakySnake as a pre-alignment filtering step reduces the execution time of Parasail by 1.2× (using 100bp_1 and 40 threads) to 28.2× (using 250bp_2 and a single thread). (3) Both SneakySnake and Parasail scale very well as the number of threads increases. We provide the exact values of all evaluation results in https://github.com/CMU-SAFARI/SneakySnake/tree/master/Evaluation%20Results.

We conclude that SneakySnake efficiently supports multithreading. Integrating SneakySnake with a state-of-the-art sequence alignment algorithm is always beneficial and reduces the end-to-end execution time by up to an order of magnitude even when using a large number of threads for both tools.

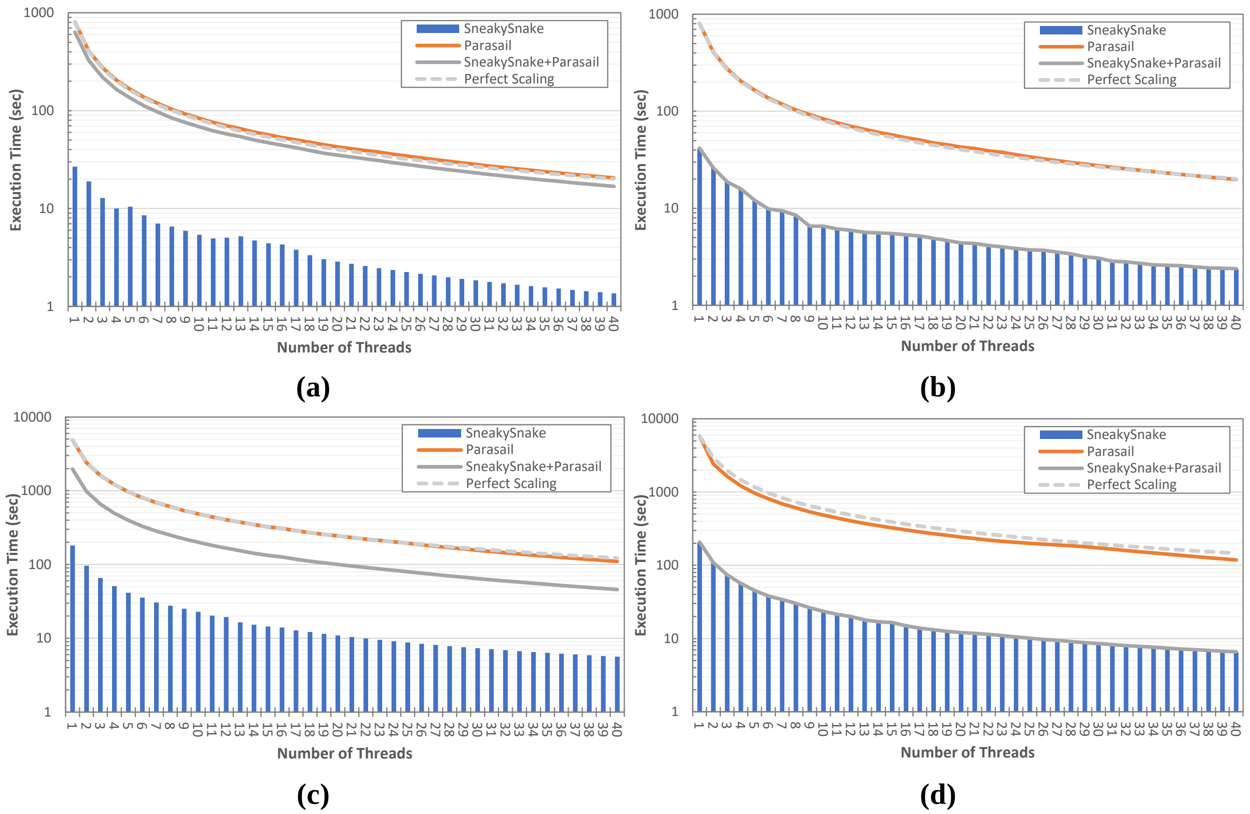


**Fig. 9: The effect of multithreading on the execution time of SneakySnake, Parasail, and SneakySnake integrated with Parasail. All y-axes are on a logarithmic scale. We use four datasets:** 100bp_1 **in (a),** 100bp_2 **in (b),** 250bp_1 **in (c), and** 250bp_2 **in (d).** 100bp_1 **and** 100bp_2 **use a sequence length (*m*) of 100 bp, while** 250bp_1 **and** 250bp_2 **use a sequence length (*m*) of 250 bp. We set the edit distance threshold (*E*) to 10% of the sequence length (i.e., *E*=10 in (a) and (b) and *E*=25 in (c) and (d)). We also provide a theoretical linear scaling of Parasail's execution time, referred to as *perfect scaling*.**

### 10.3. Evaluating the Execution Time of Filtering and Alignment Using Long Sequences

We examine the execution time of SneakySnake, Parasail, and SneakySnake integrated with Parasail using long sequences, as we show in Fig. 10. We run both SneakySnake and Parasail using two sets (10Kbp and 100Kbp) of long sequences and 40 CPU threads. We run SneakySnake with $t = y = (E+500)$, where $t$ is the width of the chip maze of each subproblem, $y$ is the number of iterations performed to solve each subproblem, and $E$ is the edit distance threshold. We choose the values of $t$ and $y$ to be less than the sequence length to prevent SneakySnake from examining the entire chip maze, which helps to achieve fast filtering at the cost of a slight increase in the number of falsely-accepted pairs (with a 0% false reject rate). We also choose the values of $t$ and $y$ to be more than $E$ to prevent the chip maze from having complete rows of obstacles based on Equation 1 in the main paper. We experimentally evaluate the effect of varying the values of $t$ and $y$ on both the accuracy and execution time of SneakySnake in https://github.com/CMU-SAFARI/SneakySnake/tree/master/Evaluation%20Results. We generate the two sets of long sequence pairs

using PBSIM (Ono *et al.*, 2013). We use Human chromosome 1 sequence (GRCh38.p13 assembly, downloaded from https://www.ncbi.nlm.nih.gov/nuccore/NC_000001.11) for the input reference sequence in PBSIM. We generate 10Kbp to have 100,000 sequence pairs, each of which is 10 Kbp long, at 30× genome coverage. 100Kbp has 74,687 sequence pairs, each of which is 100 Kbp long, at 30× genome coverage. For both sets (10Kbp and 100Kbp), we use the default error profile for the continuous long reads (CLR) in PBSIM. We use a wide range of edit distance thresholds, up to 20% of the sequence length.

Based on Fig. 10, we make two key observations. (1) Using 10Kbp and 100Kbp, SneakySnake makes Parasail significantly faster (by 58.2-708.4× and by 50.9-978.8×, respectively) than Parasail alone in detecting dissimilar pairs of long sequences, even at high edit distance thresholds (up to $E$=501 for 10Kbp and up to $E$=5010 for 100Kbp, which results in building and examining 1003 and 10021 rows, respectively, for each chip maze of the SneakySnake algorithm). (2) As the number of similar sequence pairs increases (at $E > 501$ for 10Kbp and at $E > 5010$ for 100Kbp), the benefit of integrating SneakySnake with Parasail in reducing the end-to-end execution time reduces. When Parasail examines 89% and 94% of the input sequence pairs (SneakySnake filters out the rest of the sequence pairs) of 10Kbp and 100Kbp datasets, respectively, SneakySnake provides slight or no performance benefit to the end-to-end execution time of the sequence aligner alone. This is expected, as each sequence pair that passes SneakySnake is examined unnecessarily twice (i.e., once by SneakySnake and once by Parasail). We provide the exact values of all evaluation results in https://github.com/CMU-SAFARI/SneakySnake/tree/master/Evaluation%20Results.

We conclude that SneakySnake supports multithreaded filtering for long sequences. Integrating SneakySnake with a state-of-the-art sequence alignment algorithm that supports multithreading is also beneficial and sometimes reduces the end-to-end execution time by up to two orders of magnitude.

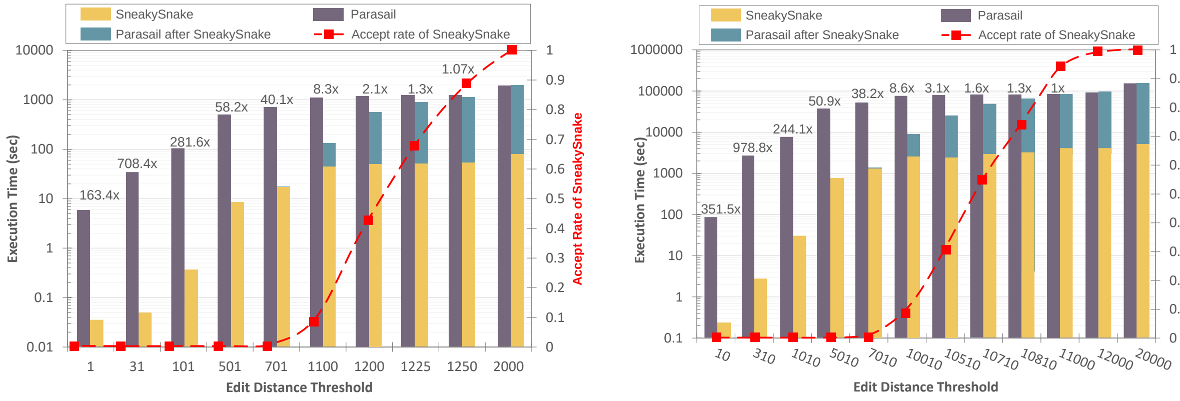


**(a)** **(b)**

**Fig. 10: The execution time of SneakySnake, Parasail, and SneakySnake integrated with Parasail using long sequences, (a) 10Kbp and (b) 100Kbp, and 40 CPU threads. The left y-axes of (a) and (b) are on a logarithmic scale. For each edit distance threshold value, we provide in the right y-axes of (a) and (b) the rate of accepted pairs (out of 100,000 pairs for 10Kbp and out of 74,687 pairs for 100Kbp) by SneakySnake that are passed to Parasail. We present the end-to-end speedup values obtained by integrating SneakySnake with Parasail.**

We examine the execution time of SneakySnake, KSW2, and SneakySnake integrated with KSW2 using long sequences, as we show in Fig. 11. KSW2 is a sequence aligner used in minimap2 (Li, 2018), a widely-used read mapper. We run KSW2 as *extz2_sse*, a global alignment implementation that is parallelized using the Intel SSE instructions. KSW2 uses the Z-drop heuristic (Suzuki and Kasahara, 2018) to improve the alignment time. We run both SneakySnake and KSW2 using a single CPU thread (as KSW2 does not support multithreading) and two datasets (10Kbp and 100Kbp). We run SneakySnake with $t = y = (E+500)$. Based on Fig. 11, we make two key observations. (1) Using 10Kbp and 100Kbp, SneakySnake is beneficial even for KSW2, a parallelized sequence aligner that uses heuristics. SneakySnake makes KSW2 significantly faster (by 8.2-64.1× and by 3.8-60.6×, respectively) than KSW2 alone in detecting dissimilar pairs of long sequences. (2) As the number of input sequence pairs passing SneakySnake increases up to 68% and 73% of the input sequence pairs of 10Kbp and 100Kbp, respectively, the benefits of integrating SneakySnake with KSW2 in reducing the end-to-end execution time reduces.

We conclude that SneakySnake supports filtering long sequence pairs and its performance scales well over a wide range of edit distance thresholds and sequence lengths.

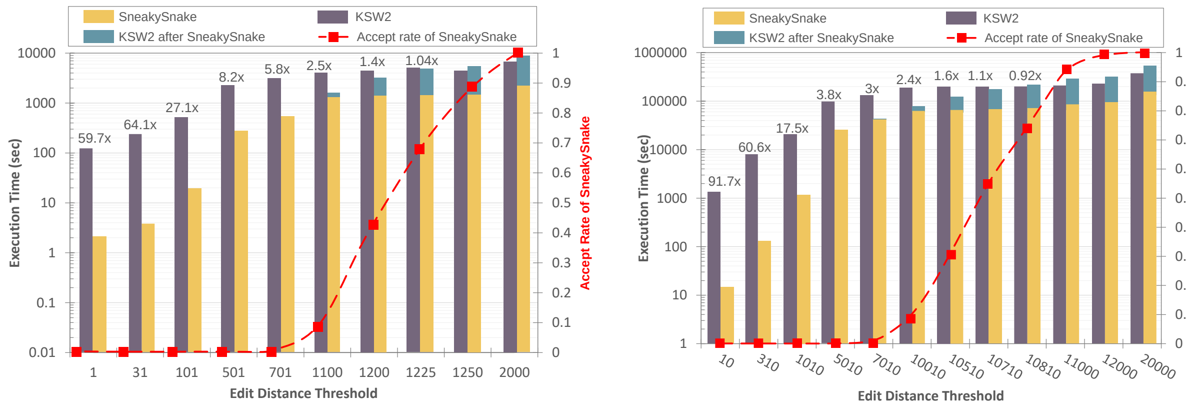


**(a)** **(b)**

**Fig. 11: The execution time of SneakySnake, KSW2, and SneakySnake integrated with KSW2 using long sequences, (a) 10Kbp and (b) 100Kbp, and a single CPU thread. The left y-axes of (a) and (b) are on a logarithmic scale. For each edit distance threshold value, we provide in the right y-axes of (a) and (b) the rate of accepted pairs (out of 100,000 pairs for 10Kbp and out of 74,687 pairs for 100Kbp) by SneakySnake that are passed to KSW2. We present the end-to-end speedup values obtained by integrating SneakySnake with KSW2.**

### 10.4. Evaluating Accuracy, Resource Analysis, and Execution Time of Snake-on-Chip

We examine 1) the number of sequence pairs that are accepted/rejected by Snake-on-Chip using 100bp_1 and 100bp_2 datasets, 2) the FPGA resource utilization for the hardware implementation of Snake-on-Chip, and 3) the execution time of Snake-on-GPU.

We build the FPGA implementation of Snake-on-Chip using a sub-matrix width of 8 columns ($t$=8) and we include 3 module instances in the design. Table 5 lists the number of accepted and rejected sequence pairs by Snake-on-Chip using the 100bp_1 and 100bp_2 datasets. We observe that Snake-on-Chip filters out 16.3% (using 100bp_1 and $E$=10) to 99.99% (using 100bp_2 and $E$=0) of input sequence pairs. This leads to a significant savings in sequence alignment time, as we show in Section 3.4. We comprehensively analyze and evaluate different sub-matrix widths in "*Effect of y & t on SneakySnake*" Excel sheet in https://github.com/CMU-SAFARI/SneakySnake/tree/master/Evaluation%20Results).

**Table 5: Number of accepted and rejected sequence pairs by Snake-on-Chip for a sequence length of 100 and under edit distance thresholds (*E*) of *E*= 0% up to *E*= 10% of the sequence length. We use 100bp_1 and 100bp_2 datasets.**

| | 100bp_1 | | | 100bp_2 | | |
|---|---|---|---|---|---|---|
| ***E* (%)** | **Accepted** | **Rejected** | **Filtering Rate (%)** | **Accepted** | **Rejected** | **Filtering Rate (%)** |
| **0** | 381'901 | 29'618'099 | 98.7270 | 11 | 29'999'989 | 99.9999 |
| **1** | 1'388'240 | 28'611'760 | 95.3725 | 20 | 29'999'980 | 99.9999 |
| **2** | 3'491'611 | 26'508'389 | 88.3613 | 25 | 29'999'975 | 99.9999 |
| **3** | 6'187'022 | 23'812'978 | 79.3766 | 29 | 29'999'971 | 99.9999 |
| **4** | 8'926'539 | 21'073'461 | 70.2449 | 40 | 29'999'960 | 99.9999 |
| **5** | 11'542'855 | 18'457'145 | 61.5238 | 126 | 29'999'874 | 99.9996 |
| **6** | 14'266'733 | 15'733'267 | 52.4442 | 480 | 29'999'520 | 99.9984 |
| **7** | 17'056'251 | 12'943'749 | 43.1458 | 1'805 | 29'998'195 | 99.9940 |
| **8** | 20'023'178 | 9'976'822 | 33.2561 | 6'078 | 29'993'922 | 99.9797 |
| **9** | 22'763'290 | 7'236'710 | 24.1224 | 17'109 | 29'982'891 | 99.9430 |
| **10** | 25'091'831 | 4'908'169 | 16.3606 | 40'697 | 29'959'303 | 99.8643 |

We examine the FPGA resource utilization for the hardware implementation of GateKeeper, Shouji, MAGNET, and Snake-on-Chip pre-alignment filters. We evaluate our four pre-alignment filters using a single FPGA chip, the Xilinx VC709 (Xilinx, 2013). We use 60 million sequence pairs, each of which is 100 bp long, from 100bp_1 and 100bp_2. We provide several hardware designs for two commonly used edit distance thresholds, 2 bp and 5 bp, for a sequence length of 100 bp. The VC709 FPGA chip contains 433,200 slice LUTs (look-up tables) and 866,400 slice registers (flip-flops). Table 6 lists the FPGA resource utilization for a single filtering unit. We make five main observations. (1) The design for a single MAGNET filtering unit requires about 10.5% and 37.8% of the available LUTs for edit distance thresholds of 2 bp and 5 bp, respectively. Hence, MAGNET can process 8 and 2 sequence pairs concurrently for edit distance thresholds of 2 bp and 5 bp, respectively, without violating the timing constraints of our hardware accelerator. (2) The design for a single Shouji filtering unit requires about 15×-21.9× fewer LUTs compared to MAGNET. This enables Shouji to achieve more parallelism over MAGNET as Shouji can have 16 filtering units within the same FPGA chip. (3) GateKeeper requires about 26.9×-53× and 1.7×-2.4× fewer LUTs compared to MAGNET and Shouji, respectively. GateKeeper can also examine up to 16 sequence

pairs at the same time on the same FPGA chip. (4) Snake-on-Chip requires 15.4×-26.6× fewer LUTs compared to MAGNET. While Snake-on-Chip requires slightly fewer LUTs compared to Shouji, it requires about 2× more LUTs compared to GateKeeper. Snake-on-Chip can also examine up to 16 sequence pairs concurrently on the same FPGA chip. (5) We observe that the hardware implementations of Shouji, MAGNET, and Snake-on-Chip require pipelining the design (i.e., shortening the critical path delay of each processing core by dividing it into stages or smaller tasks) to meet the timing constraints (the operating frequency of the accelerator is 250 MHz) and achieve more parallelism. Although we use at most 16 filtering units for GateKeeper, Shouji, and Snake-on-Chip, the Xilinx VC709 chip can still accommodate more filtering units for these three filters. However, we observe that the number of filtering units is limited by the maximum data throughput that can supply inputs to the filtering units, which is nearly 3.3 GB/s (13.3 billion bases per second) as provided by the RIFFA communication channel that feeds data into the FPGA (Jacobsen *et al.*, 2015).

**Table 6: FPGA resource usage for a single filtering unit of GateKeeper, Shouji, MAGNET, and Snake-on-Chip for a sequence length of 100 and under different edit distance thresholds (*E*).**

| | ***E* (%)** | **Slice LUT** | **Slice Register** | **No. of Filtering Units** |
|---|---|---|---|---|
| **GateKeeper** | 2 | 0.39% | 0.01% | 16 |
| | 5 | 0.71% | 0.01% | 16 |
| **Shouji** | 2 | 0.69% | 0.08% | 16 |
| | 5 | 1.72% | 0.16% | 16 |
| **MAGNET** | 2 | 10.50% | 0.80% | 8 |
| | 5 | 37.80% | 2.30% | 2 |
| **Snake-on-Chip** | 2 | 0.68% | 0.16% | 16 |
| | 5 | 1.42% | 0.34% | 16 |

We also analyze the execution time of our hardware pre-alignment filters, GateKeeper, MAGNET, Shouji, and Snake-on-Chip. For a single filtering unit, each of the four pre-alignment filters takes about 0.7233 seconds to complete examining 100bp_1 and 100bp_2, regardless the edit distance threshold used (we test it for $E$ = 0% to 5% of the sequence length). This is because these hardware architectures utilize a 250 MHz clock signal that synchronizes the entire computation. That is, increasing the edit distance threshold directly increases the number of HRTs for each SNR subproblem but does not necessarily increase the execution time as the FPGA provides a large number of LUTs that operate in parallel. Increasing the edit distance threshold is only limited by the available FPGA resource and probably the critical path delay. This is clear from the FPGA resource usage that is correlated with the filtering accuracy and the edit distance threshold. For example, the least accurate filter, GateKeeper, occupies the least amount of FPGA resources.

We conclude that Snake-on-Chip requires a reasonably small number of LUTs, which allows us to integrate a large number of filtering units that can examine a large number of sequence pairs in parallel.

### 10.5. Evaluating Execution Time and Accuracy of Snake-on-GPU

We examine 1) the end-to-end filtering time of Snake-on-GPU and 2) the number of sequence pairs that are accepted/rejected using 100bp_1 and 100bp_2 datasets. We use *cudaEventElapsedTime()* function to measure the total execution time (i.e., end-to-end filtering time), which we provide in Table 7. We make two key observations. 1) Snake-on-GPU filters out 13.3% (using 100bp_1 and *E*=10) to 99.99% (using 100bp_2 and *E*=0) of input sequence pairs. This leads to a significant savings in sequence alignment time, as we show in Section 3.4. 2) Host-GPU data transfer (sending the sequence pairs from the host to the GPU and receiving back the filtering results from the GPU) consumes 72% (using 100bp_1 and *E*=10) to 85% (using 100bp_2 and *E*=0) of the end-to-end filtering time.

**Table 7: Breakdown of Snake-on-GPU end-to-end filtering time (in seconds) and number of accepted and rejected sequence pairs by Snake-on-GPU, using NVIDIA GeForce RTX 2080Ti card, under different edit distance thresholds (*E*). We use 100bp_1 and 100bp_2 with a sequence length of 100 bp.**

| Dataset | *E* (%) | Computation Time (sec) | Data Transfer Time (sec) | End-to-End Filtering Time (sec) | Accepted | Rejected | Filtering Rate (%) |
|---|---|---|---|---|---|---|---|
| 100bp_1 | **0** | 0.0903 | 0.4818 | **0.5722** | 653'408 | 29'346'106 | 97.8204 |
| | **1** | 0.1004 | 0.4529 | **0.5534** | 2'065'683 | 27'932'871 | 93.1096 |
| | **2** | 0.1050 | 0.4530 | **0.5581** | 4'665'768 | 25'331'194 | 84.4373 |
| | **3** | 0.1097 | 0.4558 | **0.5655** | 7'601'344 | 22'393'785 | 74.6460 |
| | **4** | 0.1173 | 0.4519 | **0.5692** | 10'460'264 | 19'533'122 | 65.1104 |
| | **5** | 0.1251 | 0.4529 | **0.5781** | 13'202'659 | 16'789'361 | 55.9645 |
| | **6** | 0.1320 | 0.4597 | **0.5918** | 16'029'917 | 13'960'784 | 46.5359 |
| | **7** | 0.1579 | 0.6049 | **0.7628** | 18'836'982 | 11'152'303 | 37.1743 |
| | **8** | 0.1560 | 0.5354 | **0.6914** | 21'604'033 | 8'383'825 | 27.9461 |
| | **9** | 0.1681 | 0.4727 | **0.6408** | 24'019'045 | 5'967'465 | 19.8916 |
| | **10** | 0.1815 | 0.4636 | **0.6451** | 25'994'473 | 3'990'988 | 13.3033 |
| 100bp_2 | **0** | 0.0877 | 0.4900 | **0.5777** | 11 | 29'999'989 | 99.9999 |
| | **1** | 0.1002 | 0.4533 | **0.5535** | 22 | 29'999'978 | 99.9999 |
| | **2** | 0.1017 | 0.4518 | **0.5534** | 29 | 29'999'971 | 99.9999 |
| | **3** | 0.1024 | 0.4483 | **0.5507** | 34 | 29'999'966 | 99.9999 |
| | **4** | 0.1047 | 0.4494 | **0.5540** | 61 | 29'999'939 | 99.9998 |
| | **5** | 0.1080 | 0.4492 | **0.5572** | 292 | 29'999'708 | 99.9990 |
| | **6** | 0.1078 | 0.4548 | **0.5626** | 1'287 | 29'998'713 | 99.9957 |
| | **7** | 0.1324 | 0.6449 | **0.7773** | 4'233 | 29'995'767 | 99.9859 |
| | **8** | 0.1233 | 0.5221 | **0.6453** | 12'039 | 29'987'961 | 99.9599 |
| | **9** | 0.1302 | 0.4522 | **0.5824** | 30'176 | 29'969'824 | 99.8994 |
| | **10** | 0.1393 | 0.4537 | **0.5931** | 68'791 | 29'931'209 | 99.7707 |

### 10.6. Key Differences Between Snake-on-Chip and Snake-on-GPU

We summarize the differences between Snake-on-Chip and Snake-on-GPU in terms of 1) their ability to configure the parameter values with minimal changes, 2) energy efficiency of FPGA compared to GPU, 3) their portability from implementation on the same FPGA or GPU system architecture to implementation on another FPGA or GPU system with minimal code changes, 4) their scalability with edit distance threshold, 5) typical design effort required, 6) the market cost of a powerful FPGA compared to a powerful GPU. We provide the summary of these six key differences in Table 8. We observe that both Snake-on-Chip and Snake-on-GPU have their unique pros and cons and hence deciding on which hardware accelerator to use is left to the user's preferences and design goals.

**Table 8: A summary of the key differences between Snake-on-Chip and Snake-on-GPU.**

| | Snake-on-Chip (FPGA) | Snake-on-GPU (GPU) | Explanation |
|---|---|---|---|
| **Parameter Configurability** | ✗ | ✓ | – Snake-on-Chip requires changing the architecture at design time for each different parameter (e.g., edit distance threshold, *E*, and the width, *t*, of each subproblem) value.<br>– Snake-on-GPU is fully configurable at compile-time and run-time. |
| **Energy Efficiency** | ✓ | ✗ | – FPGA is typically more energy-efficient than GPU (Falsafi *et al.*, 2017; Chung *et al.*, 2010; Guo *et al.*, 2019). |
| **Portability** | ✓ | ✓ | – Snake-on-Chip is independent of the specific FPGA-platform as it does not rely on any vendor-specific computing element (e.g., intellectual property cores).<br>– Snake-on-GPU is independent of the specific CUDA-supported device. |
| **Scalability** | ✓ | ✓ | – The performance of Snake-on-Chip and its filtering units depends only on the clock speed and not the filtering speed (as we show in Section 10.4). For example, increasing the edit distance threshold directly increases the number of HRTs for each SNR subproblem but does not necessarily increase the execution time as the FPGA provides a large number of LUTs that operate in parallel. This makes the scalability of Snake-on-Chip to high edit distance thresholds or long sequences dependent on *only* the available FPGA resources (and probably the critical path delay) that can accommodate more filtering units. |

| | | | |
|---|---|---|---|
| | | | – The scalability of Snake-on-GPU is determined by the number of threads that can work concurrently. This makes it dependent on the filtering speed (i.e., how early a pair of sequences can be deemed dissimilar) of each thread.<br>– Given that FPGA has a large number (typically few millions) of LUTs and GPU has a large number (typically few thousands) of threads, we can consider both Snake-on-Chip and Snake-on-GPU scalable with edit distance threshold (as we also experimentally evaluate in Sections 10.4 and 10.5). |
| **Design Effort** | ✗ | ✓ | – Snake-on-Chip requires a longer design time and more design effort than Snake-on-GPU. |
| **Cost** | ✗ | ✓ | – FPGA is usually more expensive than GPU, for example, Xilinx VC709 (Xilinx 2013) is 3.6x more expensive than NVIDIA GeForce RTX 2080Ti (NVIDIA 2019b). |

**References:**


1000 Genomes Project Consortium. (2015). A global reference for human genetic variation. *Nature*, **526**(7571), 68-74.

Alkan, C., Kidd, J. M., Marques-Bonet, T., Aksay, G., Antonacci, F., Hormozdiari, F., Kitzman, J. O., Baker, C., Malig, M. and Mutlu, O. (2009). Personalized copy number and segmental duplication maps using next-generation sequencing, *Nature genetics*, **41**, 1061-1067.

Alser, M., Hassan, H., Xin, H., Ergin, O., Mutlu, O., and Alkan, C. (2017a). GateKeeper: A new hardware architecture for accelerating pre-alignment in DNAshort read mapping. *Bioinformatics*, **33**(21), 3355–3363.

Alser, M., Mutlu, O., and Alkan, C. (2017b). MAGNET: Understanding and improving the accuracy of genome pre-alignment filtering. *Transactions on Internet Research*, **13**(2), 33–42.

Alser, M., Hassan, H., Kumar, A., Mutlu, O., and Alkan, C. (2019). Shouji: A fast and efficient pre-alignment filter for sequence alignment. *Bioinformatics*, **35**(21), 4255–4263.

Alser, M., Bingöl, Z., Cali, D. S., Kim, J., Ghose, S., Alkan, C., and Mutlu, O. (2020a). Accelerating genome analysis: A primer on an ongoing journey. *IEEE Micro*, **40**(5), 65–75.

Alser, M., Rotman, J., Taraszka, K., Shi, H., Baykal, P. I., Yang, H. T.,Xue, V., Knyazev, S., Singer, B. D., Balliu, B.,et al. (2020b). Technology dictates algorithms: Recent developments in read alignment. *arXiv preprint* arXiv:2003.00110.

Chaisson, M. J. and Tesler, G. (2012). Mapping single molecule sequencing reads using basic local alignment with successive refinement (BLASR): application and theory. *BMC Bioinformatics*, **13**(1), 238.

Chu, Chris, and Wong, Yiu-Chung (2007). FLUTE: Fast lookup table based rectilinear steiner minimal tree algorithm for VLSI design, *IEEE Transactions on Computer-Aided Design of Integrated Circuits and Systems*, **27**(1), 70-83.

Chung, E. S., Milder, P. A., Hoe, J. C., and Mai, K. (2010). Single-chip heterogeneous computing: Does the future include custom logic, FPGAs, and GPGPUs?. *In 2010 43rd annual IEEE/ACM international symposium on microarchitecture* (pp. 225-236).

Daily, J. (2016). Parasail: SIMD C library for global, semi-global, and local pairwise sequence alignments. *BMC bioinformatics*, **17**(1), 81.

Dimitrakopoulos, G., Galanopoulos, K., Mavrokefalidis, C. and Nikolos, D. (2008). Low-power leading-zero counting and anticipation logic for high-speed floating point units, *IEEE transactions on very large scale integration (VLSI) systems*, **16**, 837-850.

Dijkstra, E. W. (1959). A note on two problems in connexion with graphs. *Numerische mathematik*, **1**(1), 269-271.

Falsafi, B., Dally, B., Singh, D., Chiou, D., Joshua, J. Y., and Sendag, R. (2017). FPGAs versus GPUs in data centers. *IEEE Micro*, **37**(1), 60-72.

Ghose, S., Boroumand, A., Kim, J. S., Gómez-Luna, J., and Mutlu, O. (2019). Processing-in-memory: A workload-driven perspective. *IBM Journal of Researchand Development*, **63**(6), 3–1

Gómez-Luna, J., González-Linares, J. M., Benavides, J. I. and Guil, N. (2012). Performance models for asynchronous data transfers on consumer graphics processing units, *Journal of Parallel and Distributed Computing*, **72**, 1117-1126.

Guo, L., Lau, J., Ruan, Z., Wei, P., and Cong, J. (2019). Hardware acceleration of long read pairwise overlapping in genome sequencing: A race between FPGA and GPU. *In 2019 IEEE 27th Annual International Symposium on Field-Programmable Custom Computing Machines (FCCM)* (pp. 127-135).

Hart, P. E., Nilsson, N. J., and Raphael, B. (1968). A formal basis for the heuristic determination of minimum cost paths. *IEEE transactions on Systems Science and Cybernetics*, **4**(2), 100-107.

Jacobsen, M., Richmond, D., Hogains, M., & Kastner, R. (2015). RIFFA 2.1: A reusable integration framework for FPGA accelerators. *ACM Transactions on Reconfigurable Technology and Systems (TRETS)*, **8**(4), 1-23.

Li, H. (2018). Minimap2: pairwise alignment for nucleotide sequences. *Bioinformatics*, 34(18), 3094-3100.

Mutlu, O., Ghose, S., Gómez-Luna, J., and Ausavarungnirun, R. (2019). Processing data where it makes sense: Enabling in-memory computation. *Microprocessors and Microsystems*, **67**, 28–41.

NVIDIA (2019a). CUDA C programming guide, https://docs.nvidia.com/cuda/cuda-c-programming-guide/index.html.

NVIDIA (2019b). NVIDIA GeForce RTX 2080 Ti user guide.

Ono, Y., Asai, K., andd Hamada, M. (2013). PBSIM: PacBio reads simulator—toward accurate genome assembly. *Bioinformatics*, **29**(1), 119-121.

Roy, Jarrod A., and Markov, Igor L. (2008). High-performance routing at the nanometer scale, *IEEE Transactions on Computer-Aided Design of Integrated Circuits and Systems* **27.6**, 1066-1077.

Schmidt, M., Heese, K., and Kutzner, A. (2019). Accurate high throughput alignment via line sweep-based seed processing. *Nature Communications*, **10**(1), 1939

Suzuki, H., and Kasahara, M. (2018). Introducing difference recurrence relations for faster semi-global alignment of long sequences. *BMC bioinformatics*, **19**(1), 33-47.

Šošić, M. and Šikić, M. (2017). Edlib: A C/C++ library for fast, exact sequence alignment using edit distance, *Bioinformatics*, **33**, 1394-1395.

Xilinx (2013). Virtex-7 XT VC709 connectivity kit.

Xin, H., Greth, J., Emmons, J., Pekhimenko, G., Kingsford, C., Alkan, C., and Mutlu, O. (2015). Shifted Hamming Distance: A fast and accurate SIMD-friendly filter to accelerate alignment verification in read mapping. *Bioinformatics*, **31**(10), 1553–1560.
